# Supplementary material for: Irreversibility Enhances Quantum-Enhanced Markov-Chain Monte Carlo
Source: arXiv:2606.23350 source file (2026-11-18)
Supplement: Supplementary file 1 [file SI.tex]

\documentclass[superscriptaddress,amsmath,onecolumn,amssymb,notitlepage,prl,aps]{revtex4-2}

\usepackage{newfloat,algcompatible}
\usepackage{etoolbox}
\AtBeginEnvironment{algorithm}{\noindent\hrulefill\par\nobreak\vskip-5pt}
\DeclareFloatingEnvironment[
    fileext=loa,
    listname=List of Algorithms,
    name=ALGORITHM,
    placement=tbhp,
]{algorithm}

\usepackage{graphicx,subfigure,bbm}

\usepackage{amsmath}
\usepackage{empheq}
\usepackage{tabularx}
\usepackage{amsthm}
\usepackage{physics}
\usepackage{amssymb}
\usepackage{array,bm}
\usepackage{fancyhdr}
\usepackage{color}
\usepackage{extarrows}
\usepackage{enumerate}
\usepackage[colorlinks,
            linkcolor=black,
            citecolor=black,
            urlcolor=blue
            ]{hyperref}
\usepackage{tikz}
\usetikzlibrary{shapes,arrows}

% Define block styles
\tikzstyle{decision} = [diamond, draw, fill=blue!20,
    text width=4.5em, text badly centered, node distance=3cm, inner sep=0pt]
\tikzstyle{block} = [rectangle, draw, fill=blue!20,
    text width=10em, text centered, rounded corners, minimum height=4em]
\tikzstyle{line} = [draw, -latex']
\tikzstyle{cloud} = [rectangle, draw,fill=red!20, node distance=7cm,
    minimum height=4em]

\def\(({\left(}
\def\)){\right)}
\def\[[{\left[}
\def\]]{\right]}

\newcommand{\be}{\begin{equation}}
\newcommand{\ee}{\end{equation}}
\newcommand{\bea}{\begin{eqnarray}}
\newcommand{\eea}{\end{eqnarray}}

\DeclareMathAlphabet{\varmathbb}{U}{bbold}{m}{n}

%\newcommand{\Tr}{{\rm Tr}}

%\renewcommand{\thefootnote}{\fnsymbol{footnote}}

%debut

%\bibliographystyle{apsrev4-2}
%\bibliographystyle{apsrev4-2}
%\bibliographystyle{naturemag}

\usepackage{multirow}
\usepackage{makecell}
\usepackage{booktabs}

\begin{document}
\title{Supplemental Material: Irreversibility Enhances Quantum-Enhanced Markov-Chain Monte Carlo}
%Enhancing quantum-enhanced Markov Chain Monte Carlo by breaking detailed balance}
%\title{Supplementary Information: Quantum-enhanced Markov Chain Monte Carlo without detailed balance}% Machine learning dynamical phase transitions in nonequilibrium statistical mechanics}

\author{Kefan Cao}
\altaffiliation{These authors contributed equally}
\affiliation{Institute of Fundamental and Frontier Sciences, University of Electronic Science and Technology of China, Chengdu 611731, China}
\affiliation{Yingcai Honor College, University of Electronic Science and Technology of China, Chengdu 611731, China}

\author{Zidong Cui}
\altaffiliation{These authors contributed equally}
\affiliation{Institute of Fundamental and Frontier Sciences, University of Electronic Science and Technology of China, Chengdu 611731, China}
\affiliation{School of Physics, University of Electronic Science and Technology of China, Chengdu 611731, China}

\author{Lei Wang}
\affiliation{Beijing National Laboratory for Condensed Matter Physics and Institute of Physics, Chinese Academy of Sciences, Beijing 100190, China}

\author{Ying Tang}
\email[Corresponding authors: ]{jamestang23@gmail.com}
\affiliation{Institute of Fundamental and Frontier Sciences, University of Electronic Science and Technology of China, Chengdu 611731, China}
\affiliation{School of Physics, University of Electronic Science and Technology of China, Chengdu 611731, China}
\affiliation{Key Laboratory of Quantum Physics and Photonic Quantum Information, Ministry of Education, University of Electronic Science and Technology of China, Chengdu 611731, China}
\affiliation{Non-classical Information Science Basic Discipline Research Center of Sichuan Province, University of Electronic Science and Technology of China, Chengdu 611731, China}

%\date{\today}
%\begin{abstract}
%In the Supplementary Material, we demonstrate the algorithm of learning the dynamical partition function by tracking the time evolution of the probability distribution over time. We also provide the setting of the variational autoregressive network (VAN) and details of the training. We further give the information on applying the approach to  kinetically constrained models (KCMs).  %The mathematical derivation of the Supplementary Material is in a self-consistent manner.
%\end{abstract}

\maketitle
\tableofcontents

%\section{Supplementary Material to ``Solving nonequilibrium statistical mechanics by evolving variational autoregressive networks''}

%\section{A reinforcement-learning approach to train variational autoregressive networks}

\clearpage

\section{State Encoding}

In this section, we introduce a matrix-based formulation of the Markov process, including the transition dynamics, proposal mechanism, and target distribution, all defined over a discrete state space with a consistent indexing of states. For an $n$-spin system, we represent the $i$-th state by the spin vector $\mathbf{s}_i\in\{1,-1\}^n$, where $i\in[0,2^n-1]$. We define $P$ as a $2^n\times 2^n$ left-stochastic transition matrix whose elements are given by the transition probabilities $\{P(\mathbf{s}_{j}\mid\mathbf{s}_{i})\}$. Similarly, $Q$ represents a $2^n\times 2^n$ left-stochastic matrix of proposal probabilities $\{Q(\mathbf{s}_{j}|\mathbf{s}_{i})\}$. We also define $\pi\in\mathbb{R}^{2^n}$ as the target probability vector of $\{\pi(\mathbf{s}_{i})\}$, following the same ordering convention.

Moreover, IQEMC encodes spin states into quantum computational-basis states. Supplemental Table~\ref{tab:state} summarizes this convention and assigns each state a unique integer label. 
\begin{table}[h]
\centering
\caption{Encoding convention for spin states, computational-basis states, and integer labels.}
\label{tab:state}
\begin{tabular}{ccc}
\hline
\multicolumn{3}{c}{Spin state representation} \\
\hline
State& Encoding & Integer \\
$(1,\ldots,1,1)$ & $|0\ldots00\rangle$ & $0$ \\
$(1,\ldots,1,-1)$ & $|0\ldots01\rangle$ & $1$ \\
$(1,\ldots,-1,1)$ & $|0\ldots10\rangle$ & $2$ \\
$\ldots$ & $\ldots$ & $\ldots$ \\
$(-1,\ldots,-1,-1)$ & $|1\ldots11\rangle$ & $2^n - 1$ \\
\hline
\end{tabular}
\end{table}

\section{Algorithm Details}

In this section, we present the irreversible quantum-enhanced Monte Carlo (IQEMC) framework, beginning with Markov-chain validity, followed by sampling-efficiency diagnostics and state-dependent convergence analysis, and concluding with a circuit-level implementation.

\subsection{Irreducibility and Aperiodicity}

Irreducibility and aperiodicity ensure that the stationary distribution specified by the balance condition is dynamically attained. Specifically, an irreducible finite Markov chain admits a unique stationary distribution $\pi$, and aperiodicity guarantees convergence to $\pi$ from any initial distribution~\cite{mcmt}. Once the target distribution is fixed by the global balance condition, convergence follows even when the transition matrix $P$ is too large to store or diagonalize explicitly. In this subsection, we show that the Markov chain of IQEMC is irreducible and aperiodic, thereby ensuring that the chain explores the relevant state space without becoming trapped in deterministic cycles.

To simplify the analysis, we consider only proposed transitions with nonzero proposal probability, $Q(\mathbf{s}_{j}|\mathbf{s}_{i}) \neq 0$, since transitions with $Q(\mathbf{s}_{j}|\mathbf{s}_{i}) = 0$ can never be accepted or rejected. For $Q(\mathbf{s}_{j}|\mathbf{s}_{i}) > 0$ and finite temperature $T>0$, the Metropolis acceptance probability satisfies $A(\mathbf{s}_{j}|\mathbf{s}_{i})=\min\{1,e^{-\Delta E/T}\}>0$. Hence $P(\mathbf{s}_{j}|\mathbf{s}_{i}) > 0$ for all state pairs. Since every state is reachable from every other in one step, the Markov chain is irreducible. Similarly, $Q(\mathbf{s}_{i}|\mathbf{s}_{i}) > 0$ and $A(\mathbf{s}_{i}|\mathbf{s}_{i}) = 1$. The existence of a positive self-transition for every state therefore guarantees that the Markov chain is aperiodic.

In short, positivity of the proposal probabilities, $Q(\mathbf{s}_j|\mathbf{s}_i) > 0$, guarantees both irreducibility and aperiodicity. Formally, this condition can be enforced by mixing the quantum proposal with a small uniform proposal. In practice, however, this condition is typically satisfied because the quantum dynamics assigns nonzero amplitudes to most transitions, while experimental noise further introduces nonzero weight to otherwise suppressed transitions. The resulting Markov chain therefore converges to the stationary distribution $\boldsymbol{\pi}$.

\subsection{Autocorrelation}

The spectral gap characterizes convergence through the eigenvalue spectrum of the full transition matrix. For observables, convergence can instead be quantified through the autocorrelation function (ACF), which measures the decay of correlations in a scalar observable evaluated along the Markov chain~\cite{brooks2011handbook}.

Let $X(\mathbf{s})$ be a scalar observable of a spin state, and let $X_i=X(\mathbf{s}_i)$ and $X_j=X(\mathbf{s}_j)$ denote its values at two Markov-chain samples separated by a lag $\kappa$. The ACF is:
\begin{equation}
\rho_{\kappa} = \frac{\mathrm{Cov}(X_i, X_j)}{\mathrm{Var}(X_i)},
\end{equation}
where $\rho_\kappa\in [-1,1]$ and $\rho_0 = 1$. High autocorrelation leads to redundant information between successive samples and therefore reduces sampling efficiency. Accordingly, a rapid decay of $\rho_\kappa$ toward zero indicates short memory in the chain and efficient exploration of the state space. 

Given a discrete sequence of Markov-chain Monte Carlo (MCMC) samples, the lag-$\kappa$ autocorrelation coefficient $\rho_\kappa$ is defined theoretically as:
\begin{equation}
\rho_\kappa = \frac{\mathrm{Cov}(X_i, X_j)}{\mathrm{Var}(X_i)} = \frac{\mathbb{E}[(X_i - \mu_X)(X_j - \mu_X)]}{\mathbb{E}[(X_i - \mu_X)^2]},
\end{equation}
where $\mu_X = \mathbb{E}[X_i]$ is the population mean of the scalar observable. In practice, given an MCMC sample sequence $\{\mathbf{s}^{\mathbb{T}}\}_{\mathbb{T}=1}^{N}$, define $X^{\mathbb{T}}=X(\mathbf{s}^{\mathbb{T}})$ and $\bar{X}=N^{-1}\sum_{\mathbb{T}=1}^{N}X^{\mathbb{T}}$, where $\mathbb{T}$ indexes the Monte Carlo time steps. The lag-$\kappa$ autocorrelation coefficient is estimated by:

\begin{equation}
\hat{\rho}_\kappa = \frac{ \sum_{\mathbb{T}=1}^{N-\kappa} (X^{\mathbb{T}} - \bar{X})(X^{\mathbb{T}+\kappa} - \bar{X}) }{ \sum_{\mathbb{T}=1}^{N} (X^{\mathbb{T}} - \bar{X})^2 }.
\end{equation}
Beyond the lag-wise autocorrelation function, a more global measure of sampling efficiency is the integrated autocorrelation time, denoted by $\tau_{\mathrm{int}}$, which aggregates autocorrelations over all time lags: 
\begin{equation}
\tau_{\mathrm{int}} = 1 + 2\sum_{\kappa=1}^{\infty} \rho_\kappa.
\end{equation}
A smaller $\tau_{\mathrm{int}}$ indicates faster decorrelation and hence more efficient sampling. For a chain of length $N$, the effective sample size is approximately  $N_{\mathrm{eff}} \simeq N/\tau_{\mathrm{int}}$. Thus, reducing $\tau_{\mathrm{int}}$ increases the effective sample size.

\begin{table}[!htbp]
\centering
\caption{Integrated autocorrelation time for different MCMC proposal strategies. For each system size $n$, values are reported as $\tau_{\mathrm{int,mean}} \pm \mathrm{std}$ across random instances. Smaller values indicate better sampling efficiency.
}
\label{tab:tau-int-results}
\begin{tabular}{ccccc}
\hline
$n$ & IQEMC & QEMC & annealing & uniform \\
\hline
3  & $11.53 \pm 5.22$   & $18.58 \pm 29.21$    & $16.19 \pm 35.30$     & $14.20 \pm 1.83$ \\
4  & $18.95 \pm 9.26$   & $47.72 \pm 126.36$   & $138.55 \pm 551.79$   & $28.85 \pm 4.28$ \\
5  & $24.19 \pm 11.78$  & $33.91 \pm 50.16$    & $82.17 \pm 259.45$    & $61.19 \pm 4.56$ \\
6  & $45.85 \pm 22.95$  & $23.27 \pm 22.97$    & $34.95 \pm 73.02$     & $123.52 \pm 8.05$ \\
7  & $47.42 \pm 28.32$  & $28.16 \pm 15.35$    & $40.81 \pm 41.21$     & $254.66 \pm 0.50$ \\
8  & $45.48 \pm 16.43$  & $1692.27 \pm 4540.50$ & $75554.32 \pm 230690.97$ & $429.34 \pm 95.15$ \\
9  & $79.07 \pm 62.41$  & $134.21 \pm 370.22$  & $98615.35 \pm 311709.85$ & $956.78 \pm 168.53$ \\
10 & $123.51 \pm 92.91$ & $4622.38 \pm 8219.64$ & $16502.66 \pm 23499.64$ & $2016.72 \pm 51.97$ \\
\hline
\end{tabular}
\end{table}

In our numerical evaluation, the scalar observable is the energy of a classical spin state, namely $X(\mathbf{s})=E(\mathbf{s})$. For each problem instance and proposal strategy, $\tau_{\mathrm{int}}$ is computed directly from the stationary distribution of the explicitly constructed transition matrix, eliminating finite-sampling noise and enabling a direct comparison of decorrelation efficiency across methods. Supplemental Table~\ref{tab:tau-int-results} reports the mean integrated autocorrelation time $\tau_{\mathrm{int,mean}}$ and its standard deviation across random instances for IQEMC, quantum-enhanced MCMC (QEMC), the annealing variant, and a uniform-proposal baseline. The results show that IQEMC exhibits the best overall autocorrelation performance, achieving the lowest $\tau_{\mathrm{int,mean}}$ for $n=3-5$ and $n=8-10$, and its advantage increases with system size. Moreover, IQEMC exhibits greater robustness across random instances, whereas annealing and, in some cases, QEMC show large variability. The exceptionally large $\tau_{\mathrm{int,mean}}$ values and standard deviations observed for annealing at $n=8$ and $n=9$ suggest heavy-tailed mixing-time distributions arising from rare slow-mixing instances, leading to strongly instance-dependent performance. The uniform-proposal baseline exhibits a different limitation: $\tau_{\mathrm{int,mean}}$ increases steadily with system size, reaching $2016.72$ at $n=10$, consistent with slow mixing caused by the low acceptance rate of uninformed proposals at low temperatures.

Overall, the autocorrelation analysis demonstrates that IQEMC achieves more efficient and robust sampling by suppressing long-time correlations, thereby increasing the effective sample size, particularly in larger and more challenging problem regimes.

% The uniform proposal baseline shows a different failure mode. Its $\tau_{\mathrm{int,mean}}$ grows steadily with system size, reaching $2016.72$ at $n=10$. This behavior is consistent with low-temperature Metropolis dynamics: uniformly proposed moves often connect configurations with large energy differences and are therefore rejected with high probability, causing the Markov chain to remain trapped near its current state.

% Overall, the autocorrelation analysis demonstrates that IQEMC provides a more robust and efficient MCMC sampling procedure. Its key advantage is not merely local movement between neighboring samples, but the suppression of long-time correlations captured by $\tau_{\mathrm{int}}$. Consequently, IQEMC produces a larger effective sample size under the same number of MCMC steps, particularly in the larger and more challenging problem regimes.

\subsection{Asymptotic Normalization}
\phantomsection
\label{sec:convergence_proof}

The main text constructs an irreversible transition matrix from state-dependent quantum evolutions. In this section, we show that assembling the transition matrix from state-conditioned kernels preserves normalization for typical Sherrington-Kirkpatrick (SK) model states. Following the notation in the End Matter of the main text, $M_I$ denotes the assembled irreversible transition matrix with matrix elements $P(\mathbf{s}_c\mid\mathbf{s}_r)$, where $r$ and $c$ label the row and column indices, respectively. For each state-conditioned evolution $U(\mathbf{s}_i)$, let $M(\mathbf{s}_i)$ be the corresponding transition matrix with elements $P_i(\mathbf{s}_c\mid\mathbf{s}_r)$. The matrix $M_I$ is constructed by selecting the $i$-th row of $M(\mathbf{s}_i)$, yielding $P(\mathbf{s}_c\mid\mathbf{s}_i)=P_i(\mathbf{s}_c\mid\mathbf{s}_i)$. We show that, for a typical initial state $\mathbf{s}_i$, the self-transition probability of the state-dependent transition matrix satisfies:
\begin{equation}
    P_i(\mathbf{s}_i \mid \mathbf{s}_i) \approx P(\mathbf{s}_i \mid \mathbf{s}_i).
\end{equation}
\begin{empheq}[left=\empheqlbrace]{align}
    P_i(\mathbf{s}_i \mid \mathbf{s}_i)
    &= 1-\sum_{j\neq i} P_i(\mathbf{s}_j \mid \mathbf{s}_i),\\
    P(\mathbf{s}_i \mid \mathbf{s}_i)
    &= 1-\sum_{j\neq i} P(\mathbf{s}_j \mid \mathbf{s}_i)
     = 1-\sum_{j\neq i} P_j(\mathbf{s}_j \mid \mathbf{s}_i).
\end{empheq}
It therefore suffices to show that replacing $U(\mathbf{s}_i)$ with $U(\mathbf{s}_j)$ leaves the total transition weight into $\mathbf{s}_i$ approximately unchanged, namely:

\begin{equation}
    \sum_{j\neq i}
    \left|\langle \mathbf{s}_i|U(\mathbf{s}_i)|\mathbf{s}_j\rangle\right|^2
    \approx
    \sum_{j\neq i}
    \left|\langle \mathbf{s}_i|U(\mathbf{s}_j)|\mathbf{s}_j\rangle\right|^2.
\end{equation}

\begin{equation}
    U(\mathbf{s}_i)
    =
    \mathcal{T}
    \exp\left[
    -i\int_0^{t_0} H(\gamma(\mathbf{s}_i,t))\,dt
    \right],
\end{equation}
\begin{empheq}[left=\empheqlbrace]{align}
    H(\gamma)
    &=
    \bigl(1-\gamma(\mathbf{s}_i,t)\bigr)H_{\mathrm{prob}}
    +
    \gamma(\mathbf{s}_i,t)H_{\mathrm{mix}},\\
    \gamma(\mathbf{s}_i,t)
    &=
    \gamma_0-k(\mathbf{s}_i)t.
\end{empheq}
The first display gives the time-ordered evolution operator, while the second display specifies the state-dependent Hamiltonian and schedule used in it. For notational simplicity, $\alpha$ is absorbed into $H_{\mathrm{prob}}$, which therefore denotes the rescaled Hamiltonian $\alpha H_{\mathrm{prob}}$ used throughout the circuit and numerical analyses.

To first order in the Dyson expansion~\cite{sakurai2020modern} of the time-dependent Hamiltonian, and with $\hbar=1$, the evolution operator becomes:
\begin{equation}
    U(\mathbf{s}_i)
    =
    I
    -i\left(t_0-\gamma_0t_0+\frac{1}{2}k(\mathbf{s}_i)t_0^2\right)H_{\mathrm{prob}}
    -i\left(\gamma_0t_0-\frac{1}{2}k(\mathbf{s}_i)t_0^2\right)H_{\mathrm{mix}}
    +\mathcal{O}(\gamma^2).
\end{equation}
For off-diagonal matrix elements, the contribution from $H_{\mathrm{prob}}$ vanishes in the computational basis. Therefore,
\begin{align}
    \sum_{j\neq i}
    \left|\langle \mathbf{s}_i|U(\mathbf{s}_i)|\mathbf{s}_j\rangle\right|^2
    &=
    \sum_{j\neq i}
    \left|
    -i\left(\gamma_0t_0-\frac{1}{2}k(\mathbf{s}_i)t_0^2\right)
    \langle \mathbf{s}_i|H_{\mathrm{mix}}|\mathbf{s}_j\rangle
    +\mathcal{O}(\gamma^2)
    \right|^2,\\
    \sum_{j\neq i}
    \left|\langle \mathbf{s}_i|U(\mathbf{s}_j)|\mathbf{s}_j\rangle\right|^2
    &=
    \sum_{j\neq i}
    \left|
    -i\left(\gamma_0t_0-\frac{1}{2}k(\mathbf{s}_j)t_0^2\right)
    \langle \mathbf{s}_i|H_{\mathrm{mix}}|\mathbf{s}_j\rangle
    +\mathcal{O}(\gamma^2)
    \right|^2.
\end{align}
Neglecting common matrix-element factors and higher-order corrections, the problem reduces to:

\begin{equation}
    \sum_{j\neq i} k(\mathbf{s}_i)
    \approx
    \sum_{j\neq i} k(\mathbf{s}_j).
    \label{eq:k_sum}
\end{equation}

With $N_{s}=2^n$ the total number of states, the two sides of Eq.~\eqref{eq:k_sum} read:
\begin{align}
    \mathrm{LHS}
    &=
    \sum_{j\neq i} k(\mathbf{s}_i)
     =
    (2^n-1)k(\mathbf{s}_i),\\
    \mathrm{RHS}
    &=
    \sum_{j\neq i} k(\mathbf{s}_j)
     =
    \sum_{j=0}^{2^n-1} k(\mathbf{s}_j)-k(\mathbf{s}_i).
\end{align}
Equating the two sides gives $2^n k(\mathbf{s}_i)\approx\sum_{j=0}^{2^n-1} k(\mathbf{s}_j)$, or equivalently $ k(\mathbf{s}_i) \approx
    2^{-n}\sum_{j=0}^{2^n-1} k(\mathbf{s}_j) \equiv\langle k(\mathbf{s}_j)\rangle$. The problem thus reduces to showing that $k(\mathbf{s}_j)$ concentrates around its global mean for typical states. We now consider the SK model with $n$ spins and couplings $J_{lm}\sim\mathcal{N}(0,1)$.
\begin{equation}
    E(\mathbf{s}_j)
    =
    -\sum_{l>m}J_{lm}s_{j,l}s_{j,m}
    -
    \sum_l h_l s_{j,l}.
\end{equation}
% In the thermodynamic limit, the density of states is sharply concentrated around a Gaussian bulk with mean $\langle E\rangle=0$ and variance $\sigma_E^2=\mathcal{O}(n^2)$. Hence a typical configuration has energy $E(\mathbf{s}_j)=\mathcal{O}(n)$. By contrast, the extremal energies scale as $E_0=\mathcal{O}(-n^{3/2})$ and $E_{\max}\approx -E_0$, so that the full spectral width satisfies $\Delta E=E_{\max}-E_0\approx -2E_0=\mathcal{O}(n^{3/2})$. Thus the typical energy fluctuation is asymptotically small compared with the total spectral width.

In the thermodynamic limit, the density of states is concentrated around a Gaussian bulk with mean $\langle E\rangle=0$ and variance $\sigma_E^2=\mathcal{O}(n^2)$, so that typical energies scale as $\mathcal{O}(n)$. By contrast, the spectral width scales as $\Delta E=\mathcal{O}(n^{3/2})$, since $E_0=\mathcal{O}(-n^{3/2})$ and $E_{\max}\approx -E_0$. Typical energy fluctuations are therefore asymptotically negligible relative to the full spectrum. The state-dependent coefficient of IQEMC is:
\begin{equation}
    k(\mathbf{s}_j)
    =
    \mathcal{C}
    \left[
    2^{\frac{E(\mathbf{s}_j)-E_0}{E_{\max}-E_0}}
    -1
    \right].
\end{equation}
For a typical state $\mathbf{s}_i$, 
\begin{align}
    \frac{E(\mathbf{s}_i)-E_0}{E_{\max}-E_0}\approx\frac{E(\mathbf{s}_i)-E_0}{-2E_0}=\frac{1}{2}-\frac{E(\mathbf{s}_i)}{2E_0}.
\end{align}

Since $E(\mathbf{s}_i)=\mathcal{O}(n)$ whereas $E_0=\mathcal{O}(-n^{3/2})$, the correction is asymptotically negligible, yielding $k(\mathbf{s}_i)\approx \mathcal{C}(\sqrt{2}-1)$ for typical states. It remains to estimate the global average. We have
\begin{align}
    \langle k(\mathbf{s}_j)\rangle
    &=
    \frac{\mathcal{C}}{2^n}
    \sum_j
    \left[
    2^{\frac{E(\mathbf{s}_j)-E_0}{\Delta E}}
    -1
    \right]\\
    &=
    \mathcal{C}
    \left[
    2^{-E_0/\Delta E}
    \left\langle
    2^{E(\mathbf{s}_j)/\Delta E}
    \right\rangle
    -1
    \right].
\end{align}
Using $E_{\max}\approx -E_0$, we obtain $2^{-E_0/\Delta E}\approx 2^{1/2}$. Moreover,
\begin{equation}
    \left\langle
    2^{E(\mathbf{s}_j)/\Delta E}
    \right\rangle
    =
    \left\langle
    \exp(\beta_{\mathrm{eff}}E)
    \right\rangle,
    \qquad
    \beta_{\mathrm{eff}}
    =
    \frac{\ln 2}{\Delta E}.
\end{equation}

For the Gaussian bulk, $\left\langle e^{\beta_{\mathrm{eff}}E}\right\rangle
=\exp\left(1/2\beta_{\mathrm{eff}}^2\sigma_E^2\right).$ Because $\beta_{\mathrm{eff}}=\mathcal{O}(n^{-3/2})$ and $\sigma_E^2=\mathcal{O}(n^2)$, the exponent scales as $\mathcal{O}(n^{-1})$ and vanishes in the thermodynamic limit. Hence, $\left\langle e^{\beta_{\mathrm{eff}}E}\right\rangle\to1$, $\langle k(\mathbf{s}_j)\rangle\approx \mathcal{C}(\sqrt{2}-1)$. Since both the typical-state value and the global average converge to $\mathcal{C}(\sqrt{2}-1)$, one obtains $k(\mathbf{s}_i)\approx\langle k(\mathbf{s}_j)\rangle$ for almost all states in the thermodynamic limit. Equation~\eqref{eq:k_sum} then follows asymptotically, implying
\begin{equation}
    P_i(\mathbf{s}_i \mid \mathbf{s}_i)
    \approx
    P(\mathbf{s}_i \mid \mathbf{s}_i).
\end{equation}
Thus, for typical states, the self-transition probability in $M(\mathbf{s}_i)$ is asymptotically equal to the corresponding matrix element of $M_I$.

\begin{figure}[htbp]
\centering
{\includegraphics[width=1\textwidth]{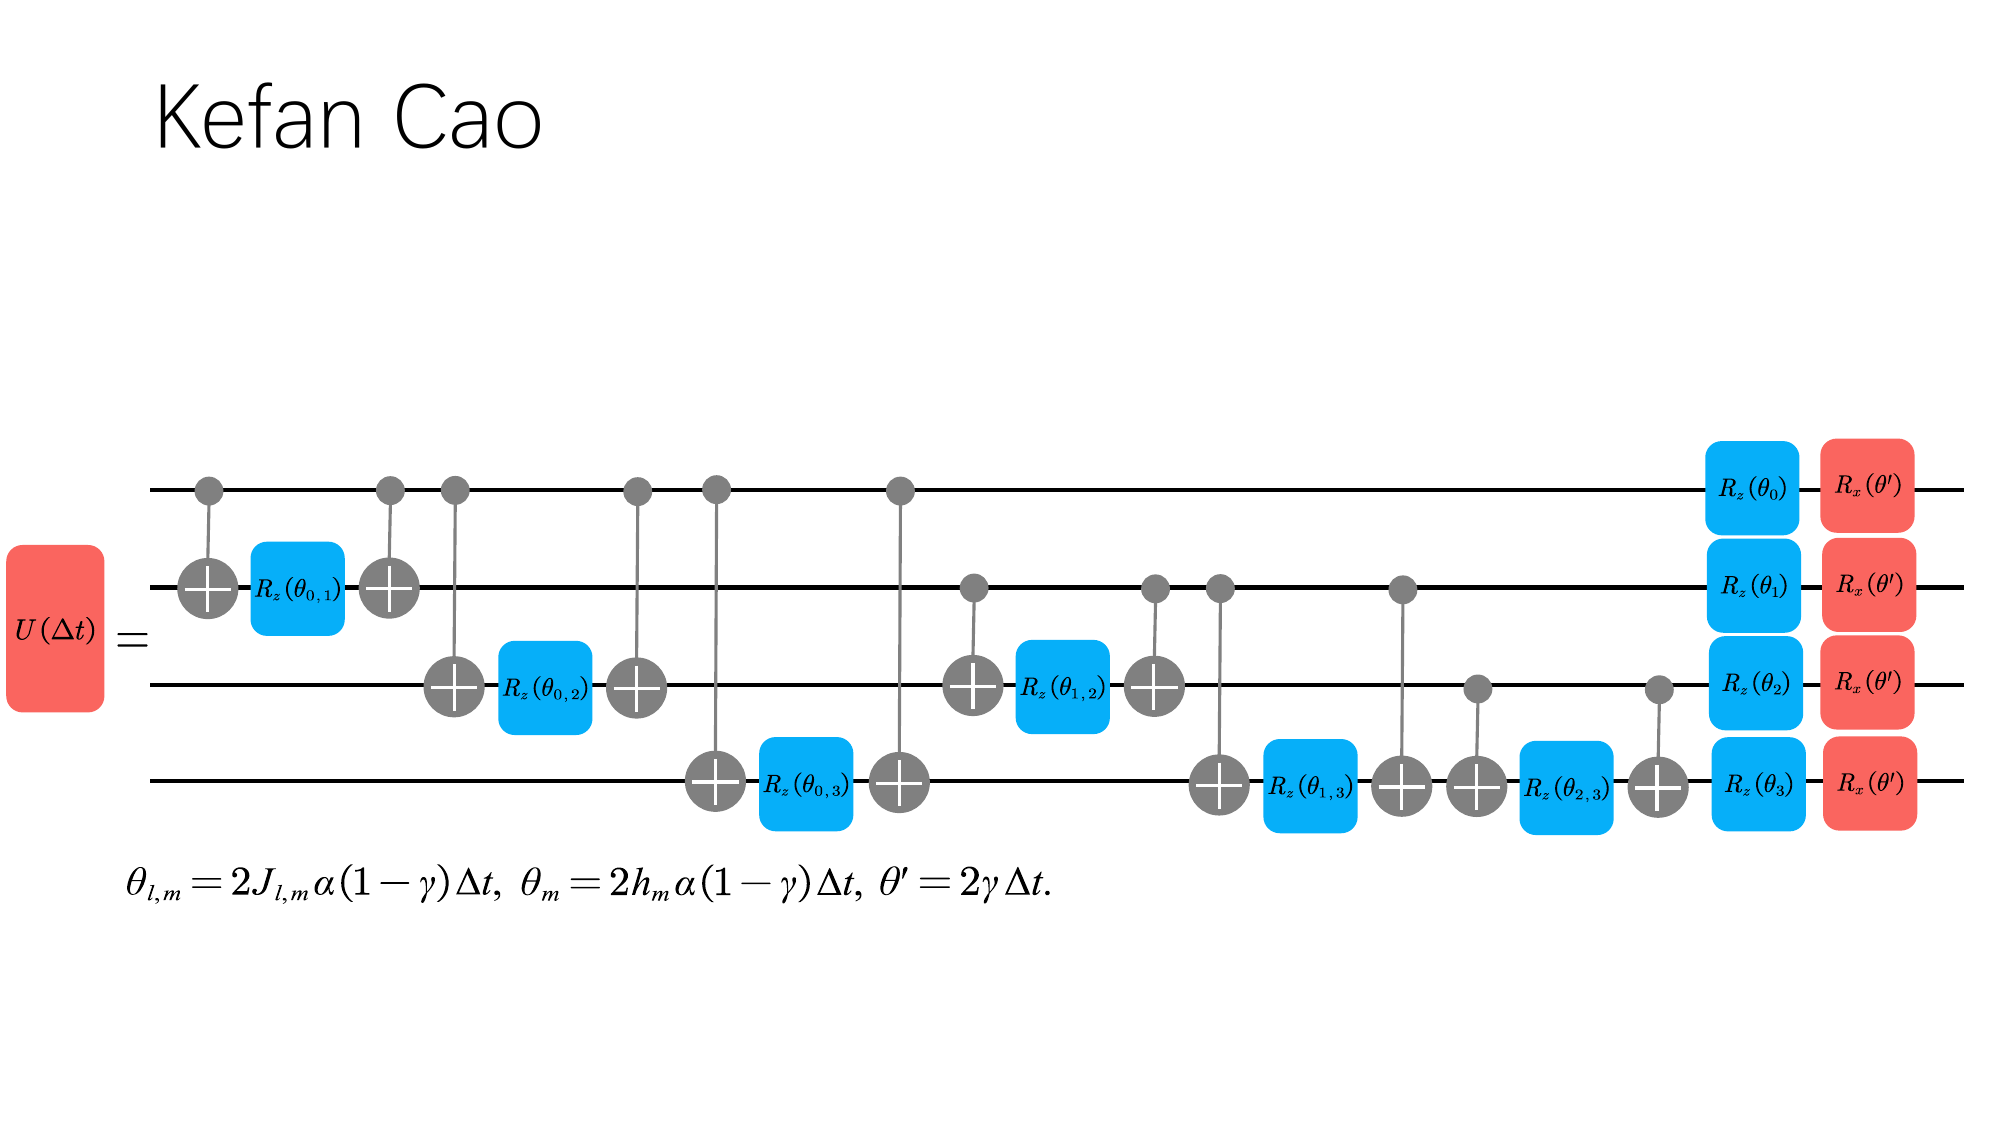}}
\caption{First-order Trotter circuit for one short-time evolution step of IQEMC. The circuit implements the operator $\exp[-i H(\mathbf{s}_i, t)\Delta t]$, with rotation angles set by the state-dependent schedule $\gamma(\mathbf{s}_i,t)=\gamma_0 - k(\mathbf{s}_i)t$, where $J_{lm}$ are pairwise couplings and $h_l$ are external fields. The $R_z$ gates encode local-field terms, controlled phase rotations encode two-body $Z_lZ_m$ couplings, and $R_x$ gates implement $H_{\mathrm{mix}}$.
}
\label{fig3}
\end{figure}

\subsection{Quantum Circuit}

In this section, we describe the circuit-level implementation of the algorithm, showing how the state-dependent Hamiltonian evolution can be decomposed into elementary gate operations available on current quantum devices.

\subsubsection{First-Order Trotter Circuits}

We first present a first-order Trotterized implementation, establishing the elementary gate primitives required for a single short-time evolution step before introducing a higher-order alternative. The time-dependent Hamiltonian for our algorithm is given by
\begin{equation}
H(\mathbf{s}_i, t) = [1 - \gamma(\mathbf{s}_i,t)]\alpha H_{\text{prob}} + \gamma(\mathbf{s}_i,t) H_{\text{mix}},
\label{hst0}
\end{equation}
where, for Boltzmann sampling of the SK model,
\begin{empheq}[left=\empheqlbrace]{align}
H_{\text{prob}} &= -\sum_{l>m} J_{lm} Z_l Z_m - \sum_{l} h_l Z_l, \\
H_{\text{mix}} &= \sum_{l} X_l, \\
\gamma(\mathbf{s}_i,t) &= \gamma_0 - k(\mathbf{s}_i) t,\\
\alpha &= \sqrt{\frac{n}{\sum_{l>m}J_{lm}^{2}+\sum_l h_l^2}}.
\end{empheq}
Here $\alpha$ is a normalization factor that rescales the problem Hamiltonian, ensuring a comparable energy scale across random Ising instances. Consequently, the relative strength of $H_{\mathrm{prob}}$ and $H_{\mathrm{mix}}$ is governed by $\gamma(\mathbf{s}_i,t)$ rather than by the sampled values of $J_{lm}$ and $h_l$.

To approximate the quantum evolution, we employ a first-order Trotter decomposition of the total evolution time $T_{\mathrm{evol}}$ into $N_{\mathrm{seg}}$ intervals of duration $\Delta t$, centered at $\{t_\nu\}_{\nu=1}^{N_{\mathrm{seg}}}$. The evolution operator is then approximated as:
\begin{align}
U(\mathbf{s}_i) \approx \prod_{\nu=1}^{N_{\text{seg}}} \exp\left(-i H(\mathbf{s}_i, t_\nu) \Delta t\right).
\end{align}
The quantum circuit implementing each $\exp\left(-iH(\mathbf{s}_i,t)\Delta t\right)$ is shown in Supplemental Figure~\ref{fig3}. It comprises single-qubit $R_z(\theta)$ and $R_x(\theta)$ rotations, as well as C-NOT gates, all of which can be decomposed into standard gate primitives supported by current quantum hardware~\cite{javadi2024quantum}.

\subsubsection{Second-Order Trotter Circuits}

The first-order construction captures the basic circuit structure, while higher-order decompositions reduce Trotter errors without changing the state-dependent control logic of IQEMC. For completeness, we present the corresponding second-order Trotter decomposition by separating single-qubit and two-body interaction terms:
\begin{align}
H_1(\mathbf{s}_i,t) &= -(1 - \gamma(\mathbf{s}_i,t))\alpha\sum_{l} h_l Z_l + \gamma(\mathbf{s}_i,t) \sum_{l} X_l,\\
H_2(\mathbf{s}_i,t) &= -(1 - \gamma(\mathbf{s}_i,t))\alpha\sum_{l>m} J_{lm}Z_l Z_m.
\end{align}
The total Hamiltonian is decomposed as $H(\mathbf{s}_i,t) = H_1(\mathbf{s}_i,t) + H_2(\mathbf{s}_i,t)$. The second-order step and full time-evolution operators are then given by:

\begin{align}
V(\mathbf{s}_i,t_\nu) &=
\exp\left(-iH_2(\mathbf{s}_i,t_\nu)\frac{\Delta t}{2}\right)
\exp\left(-iH_1(\mathbf{s}_i,t_\nu)\Delta t\right)
\exp\left(-iH_2(\mathbf{s}_i,t_\nu)\frac{\Delta t}{2}\right),\\
U(\mathbf{s}_i) &\approx \prod_{\nu=1}^{N_{\mathrm{seg}}} V(\mathbf{s}_i,t_\nu).
\end{align}

% Although we do not draw a separate circuit diagram for the second-order decomposition, the corresponding quantum circuit can be constructed directly from the gate blocks shown in Fig.~\ref{fig3}. For each time slice $t_m$, one first applies the two-body $Z_lZ_m$ interaction layer generated by $H_2(\mathbf{s}_i,t_m)$ for a half step $\Delta t/2$, then applies the single-qubit layer generated by $H_1(\mathbf{s}_i,t_m)$ for a full step $\Delta t$, and finally repeats the same two-body $H_2(\mathbf{s}_i,t_m)$ layer for another half step $\Delta t/2$. The $H_1$ layer consists of the local-field $R_z$ rotations and the transverse-field $R_x$ rotations, while the $H_2$ layer consists of the controlled phase rotations associated with the couplings $J_{lm}$. Repeating this symmetric sequence for $m=1,\ldots,N_{\mathrm{seg}}$ gives the full second-order Trotter circuit for the IQEMC proposal.

Although we do not show a separate circuit diagram for the second-order decomposition, it can be constructed from the gate blocks in Supplemental Figure~\ref{fig3}. For each time slice $t_\nu$, we apply a symmetric sequence $H_2(\Delta t/2)\!-\!H_1(\Delta t)\!-\!H_2(\Delta t/2)$, where $H_1$ contains local-field $R_z$ and transverse-field $R_x$ rotations, and $H_2$ contains controlled phase rotations encoding the couplings $J_{lm}$. Repeating this sequence for $\nu=1,\ldots,N_{\mathrm{seg}}$ yields the full second-order Trotter circuit.

\section{Numerical Details}
In this section, we describe the explicit transition-matrix construction used for the small-system numerics in the main text, enabling direct spectral-gap comparisons among IQEMC, QEMC~\cite{nature2023qe}, annealing~\cite{arai2025quantum}, and uniform proposals. We then present supplemental numerical results.

\subsection{Implementation}
%including method of calculation(delta t, delta gamma, ...), trotter decomposition, ... 

We begin with the procedure used to compute the transition matrix for a state-dependent quantum proposal. This step is the common numerical backbone for the spectral-gap, autocorrelation, and balance-condition analyses. In IQEMC, quantifying the convergence rate of the Markov chain requires constructing the transition matrix $M_{I}$. However, for our nonreversible quantum method, determining $M_{I}$ is relatively complex. We first construct $M_{I}$ from the state-dependent Hamiltonian $H(\mathbf{s}_i,t)$:
\begin{equation}
H(\mathbf{s}_i,t) = (1 - \gamma(\mathbf{s}_i,t))\alpha H_{\text{prob}} + \gamma(\mathbf{s}_i,t) H_{\text{mix}},
\label{hst}
\end{equation}
where $\gamma(\mathbf{s}_i,t)=\gamma_0-k(\mathbf{s}_i)t$. The evolution is governed by the Schr\"{o}dinger equation:
\begin{equation}
i \frac{\partial \ket{\mathbf{s}_i}}{\partial t} = H(\mathbf{s}_i,t) \ket{\mathbf{s}_i}.
\end{equation}

We denote the corresponding unitary evolution operator by $U(\mathbf{s}_i)$. The quantum measurement probability is then given by:
\begin{equation}
\Pr(\ket{\mathbf{s}_i} \rightarrow \ket{\mathbf{s}_j}) = |\bra{\mathbf{s}_j} U(\mathbf{s}_i) \ket{\mathbf{s}_i}|^2 \quad \text{for any} \quad \mathbf{s}_j \in \{\pm1\}^n, \quad \mathbf{s}_j \neq \mathbf{s}_i.
\end{equation}
The transition probability for the move $\ket{\mathbf{s}_i}\to\ket{\mathbf{s}_j}$ is $|\bra{\mathbf{s}_j}U(\mathbf{s}_i)\ket{\mathbf{s}_i}|^2$. Therefore, constructing the full transition matrix $M_I$ requires evaluating $U(\mathbf{s}_i)$ for every state $\ket{\mathbf{s}_i}$. Eq.~\eqref{hst} shows that $U(\mathbf{s}_i)$ depends on $\gamma_0$ and the total evolution time. Following the main text, we sample $t_r\in[2,20]$ and define $t_0=\min(t_r,t_z)$, with $t_z$ determined by $\gamma(\mathbf{s}_i,t_z)=0$. The unitary is written as $U(\mathbf{s}_i,\gamma_0,t_0)$. We average over $\gamma_0$ and $t_r$ to estimate the mean convergence efficiency:
\begin{equation}
    \langle U(\mathbf{s}_i)\rangle = \frac{1}{(\gamma_2 - \gamma_1)(t_2 - t_1)} \int_{\gamma_1}^{\gamma_2} \int_{t_1}^{t_2} U\bigl(\mathbf{s}_i,\gamma, \min(t_r,t_z)\bigr)  d\gamma  dt_r,
\end{equation}
where $\gamma_1 = 0.6$, $\gamma_2 = 0.8$, $t_1 = 2$, and $t_2 = 20$. This integral is difficult to calculate directly. Therefore, in practice, we use random sampling to estimate it. With $H_{\mathrm{prob}}=-\sum_{l>m}J_{lm}Z_lZ_m-\sum_l h_lZ_l$ and $H_{\mathrm{mix}}=\sum_l X_l$, the Hamiltonian $H(\mathbf{s}_i,t)$ is both time dependent and noncommuting at different times. Therefore, the evolution operator is not simply given by $e^{-iHt}$, but by the time-ordered exponential:
\begin{equation}
U(\mathbf{s}_i) \approx \prod_{\nu=1}^{N_{\mathrm{seg}}} \exp\big(-i H(\mathbf{s}_i,t_\nu) \Delta t \big),
\end{equation}
where $t_\nu=(\nu-\tfrac{1}{2})\Delta t$, with $N_{\mathrm{seg}}$ chosen to satisfy $t_0-t_{N_{\mathrm{seg}}}<\Delta t/2$. In all numerical calculations, $\Delta t=0.5$.

\subsection{Supplemental Experiment Results}
In this section, we present additional numerical results that complement the main text. These results extend the spectral-gap comparison to a broader parameter range and further support the magnetization benchmark.

\subsubsection{Spectral Gap Versus Temperature}
The main text focuses on the low-temperature regime, where metastability hinders mixing and makes sampling particularly challenging for quantum-enhanced Markov chains~\cite{orfi2024barriers}. Here we extend the comparison to additional system sizes, providing additional evidence that the IQEMC advantage is robust across system sizes. We study sampling efficiency under the Boltzmann distribution as a function of system size $n$ and temperature $T$. Beyond the $n=6$ and $T=0.1$ results shown in the main text, we present comparisons over a broader range of $n$.

In Supplemental Figure~\ref{fig:spectral-gap-temperature-supp}, we extend the temperature-dependent spectral-gap comparison to $n=4,5$, and $7$. Although the three methods exhibit distinct temperature dependences, IQEMC consistently maintains a larger spectral gap in the low-temperature regime, supporting the robustness of the advantage reported in the main text.

\begin{figure}[htbp]
\centering
\includegraphics[width=0.95\textwidth]{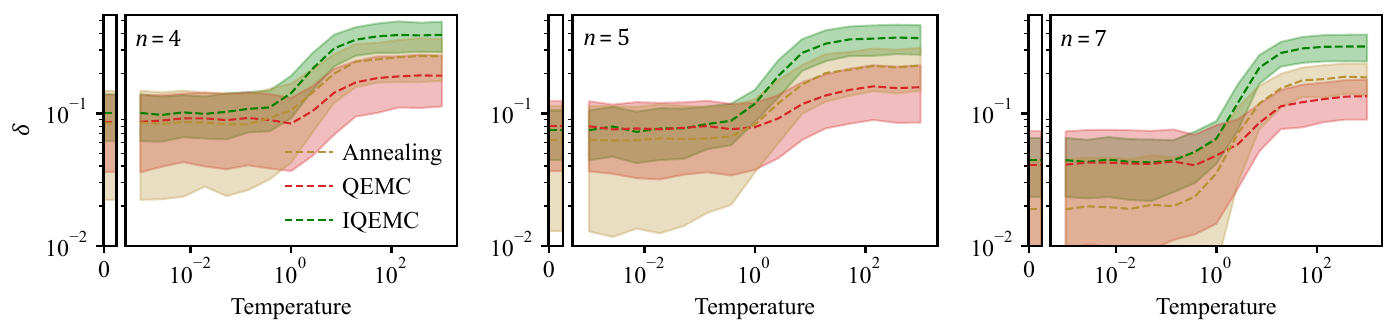}
\caption{Spectral-gap comparison versus temperature for system sizes $n=4,5$, and $7$ at $\mathcal{C}=0.15$. Across these system sizes, IQEMC maintains a larger spectral gap than annealing and QEMC in the low-temperature regime, extending the benchmark presented in the main text.}
\label{fig:spectral-gap-temperature-supp}
\end{figure}

\subsubsection{Magnetization Estimation}
Spectral-gap improvements should translate into more accurate estimates of physical observables. To test the generality of this behavior, we compare the proposal strategies across a broader set of target distributions generated from random $6$-spin Ising Hamiltonians at different temperatures. For each target Boltzmann distribution, we estimate the average magnetization and compare the convergence of IQEMC, QEMC, and uniform proposals under a fixed sampling budget. This broader benchmark tests the robustness of observable-estimation accuracy across different energy landscapes and temperatures.

% Supplemental Figure~\ref{fig:sup-mag} shows a representative additional instance in which the target Boltzmann distribution has a relatively large average magnetization. In this case, the difference between the sampling strategies becomes more pronounced: IQEMC approaches the theoretical magnetization more rapidly than both QEMC and the uniform proposal baseline. This behavior is consistent with the main-text results and further illustrates that the energy-adaptive irreversible proposal can provide a clearer advantage when the observable is strongly biased by the target distribution.

Supplemental Figure~\ref{fig:sup-mag} shows a representative instance with a relatively large average magnetization. IQEMC converges to the theoretical value more rapidly than QEMC and uniform proposals, consistent with the main-text results. The advantage is particularly evident when the target distribution is strongly biased.
\begin{figure}[t]
\centering
\includegraphics[width=0.95\textwidth]{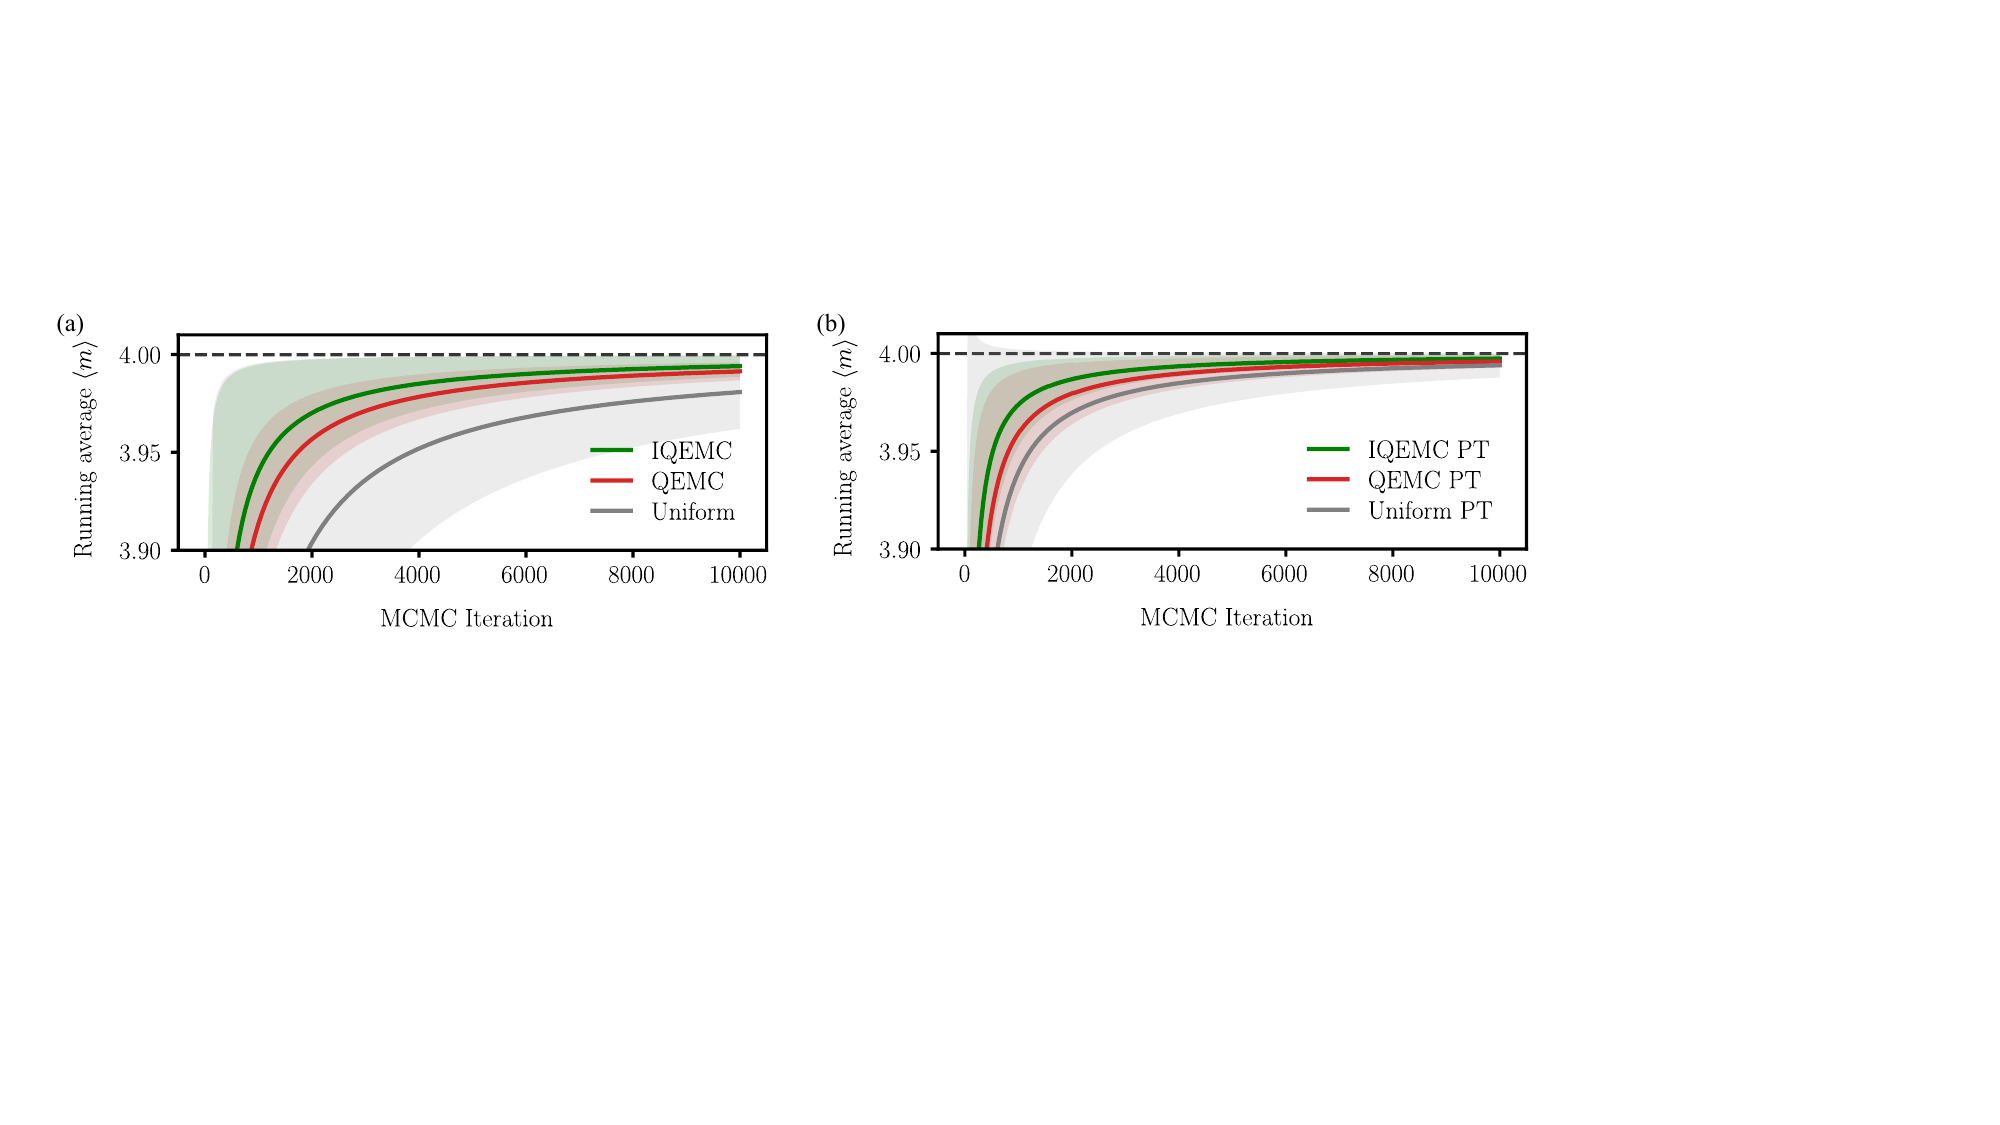}
\caption{Convergence of magnetization for a target distribution with a relatively large average magnetization at $T=0.1$ and $\mathcal{C}=0.15$. Convergence of the estimated magnetization is shown for IQEMC, QEMC, and the uniform proposal under the same sampling budget. IQEMC converges more rapidly to the theoretical value, with a more pronounced advantage in this strongly magnetized regime.}
\label{fig:sup-mag}
\end{figure}

\begin{table}[!htpb]
\centering
\caption{Numerical residuals of the mixed-column normalization condition $\left|\sum_j P_j(\mathbf{s}_j|\mathbf{s}_i)-1\right|$.}
\label{tab:mixed_column_normalization}
\begin{tabular}{c|ccc}
\hline
$n$ & Annealing & IQEMC & QEMC \\
\hline
3  & $1.65\times 10^{-17}$ & $1.49\times 10^{-17}$ & $1.65\times 10^{-17}$ \\
4  & $2.45\times 10^{-17}$ & $2.08\times 10^{-17}$ & $2.07\times 10^{-17}$ \\
5  & $3.20\times 10^{-17}$ & $2.61\times 10^{-17}$ & $3.17\times 10^{-17}$ \\
6  & $3.42\times 10^{-17}$ & $2.81\times 10^{-17}$ & $3.70\times 10^{-17}$ \\
7  & $4.59\times 10^{-17}$ & $3.50\times 10^{-17}$ & $4.23\times 10^{-17}$ \\
8  & $5.70\times 10^{-17}$ & $4.32\times 10^{-17}$ & $5.64\times 10^{-17}$ \\
9  & $7.88\times 10^{-17}$ & $5.78\times 10^{-17}$ & $7.51\times 10^{-17}$ \\
10 & $1.05\times 10^{-16}$ & $7.58\times 10^{-17}$ & $1.01\times 10^{-16}$ \\
\hline
\end{tabular}
\end{table}

\subsection{Numerical Verification of Global Balance}
The analytical analysis yields a mixed-column normalization condition. In this section, we verify this condition numerically in the benchmark implementation. In Section~\hyperref[sec:convergence_proof]{Asymptotic Normalization}, we clarify this point by explicitly deriving the condition. For the assembled transition matrix, we have $P(\mathbf{s}_j|\mathbf{s}_i)=P_i(\mathbf{s}_j|\mathbf{s}_i)$. Hence, the global balance requires
\begin{equation}
\sum_j \pi(\mathbf{s}_j)P_j(\mathbf{s}_i|\mathbf{s}_j)=\pi(\mathbf{s}_i).
\end{equation}
Using detailed balance of each fixed matrix $M(\mathbf{s}_j)$, this becomes
\begin{equation}
\sum_j \pi(\mathbf{s}_j)P_j(\mathbf{s}_i|\mathbf{s}_j)
=
\pi(\mathbf{s}_i)\sum_j P_j(\mathbf{s}_j|\mathbf{s}_i).
\end{equation}
Therefore, exact global balance of $M_I$ requires the mixed-column condition
\begin{equation}
\sum_j P_j(\mathbf{s}_j|\mathbf{s}_i)=1.
\end{equation}
This condition does not follow automatically from the detailed balance of each fixed matrix, since the summation mixes elements from different state-dependent transition matrices. We numerically verify the mixed-column normalization condition by computing the mean residual $\epsilon=\left|\sum_j P_j(\mathbf{s}_j|\mathbf{s}_i)-1\right|$. As shown in the Supplemental Table~\ref{tab:mixed_column_normalization}, the residuals for annealing, IQEMC, and QEMC are all at the level of numerical precision, confirming that the mixed-column normalization condition is satisfied in IQEMC.

\section{Discussion of the Spectral Gap for Non-Reversible Chains}
IQEMC deliberately violates detailed balance, rendering the conventional spectral-gap definition for reversible Markov chains inapplicable. This feature is central to non-reversible acceleration, where spectral modifications can enhance relaxation~\cite{vdbc,claudon2025quantum}. We show that the real part of the subleading eigenvalue associated with the stationary-distribution-weighted Markov generator governs relaxation and underlies the convergence metric used in the main text.

\subsection{Relaxation Time and Mixing Time}
In the continuous-time master-equation framework, the connection between eigenvalues and relaxation is explicit. The same rationale motivates the discrete transition-matrix diagnostic used in the numerical comparisons.

Consider the irreducible Markov process described by the master equation $d\eta_{i}(t)/dt=\sum_{j = 1}^{N_s}Q(\mathbf{s}_i|\mathbf{s}_j)\eta_{j}(t)-\sum_{j = 1}^{N_s}Q(\mathbf{s}_j|\mathbf{s}_i)\eta_{i}(t)$. Here $\eta_i(t)$ is the probability of state $i$ at time $t$, and $Q(\mathbf{s}_j|\mathbf{s}_i)$ is the transition rate from state $\mathbf{s}_i$ to state $\mathbf{s}_j$. The stationary distribution $\pi(\mathbf{s}_i)$ satisfies the balance condition, $0=\sum_{j=1}^{N_s}Q(\mathbf{s}_i|\mathbf{s}_j)\pi(\mathbf{s}_j)-\sum_{j=1}^{N_s}Q(\mathbf{s}_j|\mathbf{s}_i)\pi(\mathbf{s}_i)$, which ensures relaxation to equilibrium. The master equation can then be rewritten as: 
\begin{equation}
\frac{dR_{i}(t)}{dt}=\sum_{j = 1}^{N_s}W_{ij}R_{j}(t),
\end{equation} 
where $W_{ij}=\pi(\mathbf{s}_i)^{-1/2}Q(\mathbf{s}_i|\mathbf{s}_j)\pi(\mathbf{s}_j)^{1/2}$ ($i\neq j$), $W_{ii}=-\sum_{j(\neq i)}Q(\mathbf{s}_j|\mathbf{s}_i)$, and $R_i(t)=\eta_i(t)/\sqrt{\pi(\mathbf{s}_i)}$~\cite{vdbc}. The matrix $W$ is termed the stationary-distribution-weighted Markov generator, reflecting that its entries are not transition probabilities. Instead, $W$ is constructed from the transition rates $Q(\mathbf{s}_j|\mathbf{s}_i)$ through a stationary-distribution weighting and governs the evolution of the weighted probability vector $\vec{R}(t)$.

In vector form, the master equation reads $d\vec{R}(t)/dt=W\vec{R}(t)$, with the solution $\vec{R}(t)=e^{Wt}\vec{R}(0)$, where $\vec{\eta}(t)$ denotes the probability distribution of the sampled states and $\vec{R}(t)$ is the corresponding weighted probability vector.

Next, we consider the eigenvalues of the stationary-distribution-weighted Markov generator $W$. Since there are $N_s=2^n$ states, its eigenvalues are $\lambda_1,\lambda_2,\ldots,\lambda_{N_s}$ (sorted from largest to smallest), with corresponding eigenvectors $v_1,v_2,\ldots,v_{N_s}$. The largest eigenvalue $\lambda_1$ of $W$ is usually $0$, and the corresponding eigenvector is the steady-state distribution. Expanding the initial condition in the eigenbasis yields:
\begin{align}
\vec{R}(0) &= c_1 v_1 + c_2 v_2 + \cdots + c_{N_s} v_{N_s},\\
\vec{R}(t) &= c_1 e^{\lambda_1 t} v_1 + c_2 e^{\lambda_2 t} v_2 + \cdots + c_{N_s} e^{\lambda_{N_s} t} v_{N_s}.
\end{align}
The stationary mode associated with $\lambda_1=0$ does not decay, leaving the long-time relaxation governed by the subleading eigenvalue $\lambda_2$. The decay rate is therefore set by $\Re(\lambda_2)$, where $\Re$ and $\Im$ denote the real and imaginary parts, respectively:
\begin{equation}
\vec{R}(t) \approx c_1 v_1 + c_2 e^{\lambda_2 t} v_2 = c_1 v_1 + c_2 e^{-|\Re(\lambda_2)| t}e^{i\Im(\lambda_2) t} v_2.
\end{equation}
When $t$ is large and the sampling is close to convergence, the deviation from the steady component satisfies $|\vec{R}(t)-c_1 v_1|\le \varepsilon_{\mathrm{tol}}$, where $\varepsilon_{\mathrm{tol}}$ is a scalar convergence tolerance. This gives:
\begin{equation}
t\ge \frac{|\ln(\varepsilon_{\mathrm{tol}})|}{|c_2\Re(\lambda_2)|}.
\end{equation}
Accordingly, we define $\delta=|\Re(\lambda_2)|$ as the relaxation-rate metric for non-reversible chains. This result requires only the balance condition and therefore extends beyond detailed-balance dynamics. For reversible chains, $\delta$ coincides with the conventional spectral gap.

\clearpage
\bibliography{bib}

\end{document}
